# Supplementary material for: Computing data for Levin-Wen with defects
Source: arXiv:1907.06692 source file (2020-05-26)

$V_1$

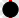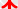

$V_2$

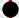

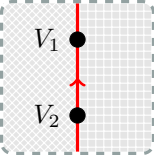

Supplement: Supplementary file 1 [file vertical_fusion_appendix_LHS.pdf]
