# Supplementary material for: Computing data for Levin-Wen with defects
Source: arXiv:1907.06692 source file (2020-05-26)
Supplement: Supplementary file 2 [file vertical_fusion_appendix_RHS.pdf]

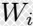

$W_i$

$W_i$

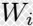

The diagram features a vertical red line that spans the entire height of the image. At the top and bottom of this line are red arrows pointing outwards, away from the center. A solid black circle is positioned exactly in the middle of the red line. To the left of this black circle, the text  $W_i$  is written in a black, serif font. The background is divided into two distinct grid patterns by the red line. The area to the left of the line is filled with a fine, light gray grid. The area to the right of the line is filled with a coarser, light gray grid. The entire image is framed by a dark gray border with rounded corners.
